# Supplementary material for: Agile Actions with a Centaur-Type Humanoid: A Decoupled Approach
Source: arXiv:2103.07183 source file (2021-03-12)
Supplement: Supplementary file 1 [file appendix_cmm.tex]

\section{Centroidal Momentum Matrix Computation}
Consider a generic humanoid robot with $n$ degrees of freedom (DoFs). Its configuration can be expressed by:
\begin{equation}
    \bm{q} = \begin{bmatrix} \bm{q}_{fb} \\ \bm{q}_a \end{bmatrix} \in \mathbb{R}^{d+n},
\end{equation}
with $\bm{q}_{fb} \in \mathbb{R}^d$ and $\bm{q}_a \in \mathbb{R}^n$.
Here, the $\bm{q}_{fb}$ is used to parameterize the 6D pose of the floating-base (FB), e.g. by using a virtual chain ($d = 6$) or by using a position and a quaternion for the orientation ($d = 7$).

If we model the floating-base pose through the virtual chain, the joint space velocities of the humanoid robot can be expressed as:
\begin{equation}
    \bm{\dot{q}} = \begin{bmatrix}\bm{\dot{q}}_{fb} \\ \bm{\dot{q}}_a \end{bmatrix} \in \mathbb{R}^{n+6},
\end{equation}
as well its joint space accelerations: $\bm{\ddot{q}} = \left[ \bm{\ddot{q}}_{fb}^\top \\ \bm{\ddot{q}}_a^\top \right]^{\top} \in \mathbb{R}^{n+6}$.
The dynamic model of the floating-base robot in contact with the environment (with $k$ number of contacts) can be written as:
\begin{equation}
    \bm{M}(\bm{q})\bm{\ddot{q}} + \bm{C}(\bm{q}, \bm{\dot{q}})\bm{\dot{q}} + \bm{g}(\bm{q}) = \bm{S}\bm{\tau} + \bm{J}_c^{\top}\bm{F}_c,
    \label{eq:dynamic_model}
\end{equation}
with $\bm{M}(\bm{q}) \in \mathbb{R}^{n+6 \times n+6}$ the generalized inertia matrix, $\bm{C}(\bm{q}, \bm{\dot{q}})\bm{\dot{q}} \in \mathbb{R}^{n+6}$ the vector accounting for Coriolis and centrifugal terms, $\bm{g}(\bm{q}) \in \mathbb{R}^{n+6}$ the vector of gravitational terms, $\bm{\tau} \in \mathbb{R}^n$ the vector of joint space torques, $\bm{S} = \left[ \bm{0}_{n \times 6}^{\top} \quad \bm{I}_{n \times n} \right]^{\top} \in \mathbb{R}^{n+6 \times n}$ is a selection matrix which impose \emph{underactuation} on the floating base joint torques, $\bm{J}_c \in \mathbb{R}^{n+6 \times k\cdot6}$ are the stacked contacts jacobians and $\bm{F}_c \in \mathbb{R}^{k\cdot6}$ are the contact forces\footnote{Notice that the floating base dynamics~\eqref{eq:dynamic_model} is constrained by $k$ kinematics constraints in the form $\bm{J}_c\bm{\ddot{q}} + \bm{\dot{J}}_c\bm{\dot{q}} = \bm{0}$}.

We can extract the first $6$ rows from~\eqref{eq:dynamic_model} which accounts for the dynamics of the floating base:
\begin{equation}
    \bm{M}_{fb}(\bm{q})\bm{\ddot{q}} + \bm{C}_{fb}(\bm{q}, \bm{\dot{q}})\bm{\dot{q}} + \bm{g}_{fb}(\bm{q}) = \bm{J}_{fb,c}^{\top}\bm{F}_c = \bm{\Gamma},
    \label{eq:fb_dynamic_model}
\end{equation}
with $\bm{M}_{fb} \in \mathbb{R}^{6 \times n+6}$, $\bm{C}_{fb}(\bm{q}, \bm{\dot{q}})\bm{\dot{q}} \in \mathbb{R}^{6}$, $\bm{g}_{fb}(\bm{q}) \in \mathbb{R}^6$ and $\bm{J}_{fb,c}^{\top} \in \mathbb{R}^{6 \times k\cdot6}$. Notice that in~\eqref{eq:fb_dynamic_model}, we assume a \emph{fictious} joint vector of torques acting at the floating base virtual chain:
\begin{equation}
    \bm{\Gamma} = \bm{J}_{fb,c}^{\top}\bm{F}_c.
    \label{eq:virtual_torques}
\end{equation}

We can compute the equivalent wrench at the floating base $\bm{F}_{fb}$\footnote{Assuming $\mathbf{J}_{fb}$ invertible}:
\begin{equation}
    \bm{F}_{fb} = \mathbf{J}_{fb}^{-\top}\bm{\Gamma},
\end{equation}
with $\mathbf{J}_{fb} \in \mathbb{R}^{6 \times 6}$ the Jacobian of the virtual chain, and express it w.r.t. the Center of Mass (CoM) of the system:
\begin{equation}
    \bm{F}_{CoM} = {^{CoM}\bm{X}_{fb}} \bm{F}_{fb} = {^{CoM}\bm{X}_{fb}}\mathbf{J}_{fb}^{-\top}\bm{\Gamma},
\end{equation}
with ${^{CoM}\bm{X}_{fb}}$ the adjoint matrix which change application point of $\bm{F}_{fb}$.
Premultiplying equation~\eqref{eq:fb_dynamic_model} by the term ${^{CoM}\bm{X}_{fb}}\mathbf{J}_{fb}^{-\top}$ leads to:
\begin{equation}
    \bm{A}(\bm{q})\bm{\ddot{q}} + \bm{\dot{A}}(\bm{q}, \bm{\dot{q}})\bm{\dot{q}} = \bm{F}_{CoM} - \bm{G}(\bm{q}),
    \label{eq:centroidal_dynamics}
\end{equation}
where:
\begin{equation}
    \bm{A}(\bm{q}) = {^{CoM}\bm{X}_{fb}}\mathbf{J}_{fb}^{-\top}\bm{M}_{fb}(\bm{q}),
    \label{eq:centroidal_momentum_matrix}
\end{equation}
is the Centroidal Momentum Matrix (CMM),
\begin{equation}
    \bm{\dot{A}}(\bm{q}, \bm{\dot{q}}) = {^{CoM}\bm{X}_{fb}}\mathbf{J}_{fb}^{-\top}\bm{C}_{fb}(\bm{q}, \bm{\dot{q}}),
\end{equation}
is the derivative of the CMM and 
\begin{equation}
    \bm{G}(\bm{q}) = {^{CoM}\bm{X}_{fb}}\mathbf{J}_{fb}^{-\top}\bm{g}_{fb}(\bm{q}).
\end{equation}
A similar computation for the CMM can be found in~\cite{wensing2016improved}.

For the Newton’s equations of motion, we can write:
\begin{equation}
    \bm{F}_{CoM} - \bm{G}(\bm{q}) = \bm{\dot{h}},
\end{equation}
with $\bm{\dot{h}} \in \mathbb{R}^6$ the time derivative of the system's centroidal momentum. 
We an use the CMM to compute the centroidal momentum of the system:
\begin{equation}
    \bm{h} = \bm{A}(\bm{q})\bm{\dot{q}}.
    \label{eq:centroidal_momentum_constraint}
\end{equation}
